# Supplementary material for: Offline Inverse Constrained Reinforcement Learning for Safe-Critical Decision Making in Healthcare
Source: arXiv:2410.07525 source file (2024-10-14)
Supplement: Supplementary file 1 [file method_experience_appendix.tex]

\subsection{The Limitations of the Markov Property in Healthcare Environments \label{B1}}

\begin{figure}[h]
    \centering
    \includegraphics[width=0.5\textwidth,keepaspectratio]{figure/limitation_mp.pdf}
    \caption{Distribution of Vaso in the same state S.}
    \label{fig:custom_cost_q}
\end{figure}
